# Supplementary material for: A Hybrid Stochastic Policy Gradient Algorithm for Reinforcement Learning
Source: arXiv:2003.00430 source file (2020-09-21)
Supplement: Supplementary file 1 [file 133-supp.pdf]

## SUPPLEMENTARY DOCUMENT

# A Hybrid Stochastic Policy Gradient Algorithm for Reinforcement Learning

This supplementary document presents the full proofs of technical results presented in the main text. It also provides the details of our configurations for numerical experiments in Section 5.

## A Convergence Analysis

We note that the original idea of using hybrid estimators has been proposed in our working paper (Tran-Dinh et al., 2019b). In this work, we have extended this idea as well as the proof techniques for stochastic optimization in Tran-Dinh et al. (2019b) into reinforcement learning settings. We now provide the full analysis of Algorithm 1 and 2. We first prove a key property of our new hybrid estimator for the policy gradient  $\nabla J(\theta)$ . Then, we provide the proof of Theorem 4.1 and Corollary 4.1.

### A.1 Proof of Lemma 4.1: Bound on the Variance of the Hybrid SPG Estimator

Part of this proof comes from the proof of Lemma 1 in Tran-Dinh et al. (2019b). Let  $\mathbb{E}_{\mathcal{B}, \hat{\mathcal{B}}}[\cdot] := \mathbb{E}_{\tau, \hat{\tau} \sim p_{\theta_t}}[\cdot]$  be the total expectation. Using the independence of  $\tau$  and  $\hat{\tau}$ , taking the total expectation on (4), we obtain

$$\begin{aligned} \mathbb{E}_{\mathcal{B}, \hat{\mathcal{B}}}[v_t] &= \beta v_{t-1} + \beta [\nabla J(\theta_t) - \nabla J(\theta_{t-1})] + (1 - \beta) \nabla J(\theta_t) \\ &= \nabla J(\theta_t) + \beta [v_{t-1} - \nabla J(\theta_{t-1})], \end{aligned}$$

which is the same as (5).

To prove (6), we first define  $u_t := \frac{1}{B} \sum_{\hat{\tau} \in \hat{\mathcal{B}}_t} g(\hat{\tau}|\theta_t)$  and  $\Delta u_t := u_t - \nabla J(\theta_t)$ . We have

$$\begin{aligned} \|\Delta v_t\|^2 &= \beta^2 \|\Delta v_{t-1}\|^2 + \frac{\beta^2}{B^2} \left\| \sum_{\tau \in \mathcal{B}_t} \Delta g(\tau|\theta_t) \right\|^2 + (1 - \beta)^2 \|\Delta u_t\|^2 + \beta^2 \|\nabla J(\theta_{t-1}) - \nabla J(\theta_t)\|^2 \\ &\quad + \frac{2\beta^2}{B} \sum_{\tau \in \mathcal{B}_t} (\Delta v_{t-1})^\top [\Delta g(\tau|\theta_t)] + 2\beta^2 (\Delta v_{t-1})^\top [\nabla J(\theta_{t-1}) - \nabla J(\theta_t)] \\ &\quad + 2\beta(1 - \beta) (\Delta v_{t-1})^\top [u_t - \nabla J(\theta_t)] + \frac{2\beta(1 - \beta)}{B} \sum_{\tau \in \mathcal{B}_t} [\Delta g(\tau|\theta_t)]^\top (\Delta u_t) \\ &\quad + \frac{2\beta^2}{B} \sum_{\tau \in \mathcal{B}_t} (\Delta g(\tau|\theta_t))^\top [\nabla J(\theta_{t-1}) - \nabla J(\theta_t)] + 2\beta(1 - \beta) (\Delta u_t)^\top [\nabla J(\theta_{t-1}) - \nabla J(\theta_t)]. \end{aligned}$$

Taking the total expectation and note that  $\mathbb{E}_{\hat{\mathcal{B}}}[u_t] := \mathbb{E}_{\hat{\tau} \sim p_{\theta_t}}[u_t] = \nabla J(\theta_t)$  and  $\mathbb{E}_{\hat{\mathcal{B}}}[\|u_t - \nabla J(\theta_t)\|^2] \leq \frac{1}{B^2} \sum_{\hat{\tau} \in \hat{\mathcal{B}}} \mathbb{E}[\|g(\hat{\tau}|\theta_t) - \mathbb{E}[g(\hat{\tau}|\theta_t)]\|^2] = \frac{\sigma^2}{B}$ , we get

$$\begin{aligned} \mathbb{E}_{\mathcal{B}, \hat{\mathcal{B}}}[\|\Delta v_t\|^2] &= \beta^2 \|\Delta v_{t-1}\|^2 + \frac{\beta^2}{B^2} \mathbb{E}_{\mathcal{B}} \left[ \left\| \sum_{\tau \in \mathcal{B}_t} \Delta g(\tau|\theta_t) \right\|^2 \right] + (1 - \beta)^2 \mathbb{E}_{\hat{\mathcal{B}}}[\|\Delta u_t\|^2] \\ &\quad - \beta^2 \|\nabla J(\theta_{t-1}) - \nabla J(\theta_t)\|^2 \\ &\leq \beta^2 \|\Delta v_{t-1}\|^2 + \frac{\beta^2}{B^2} \sum_{\tau \in \mathcal{B}_t} \mathbb{E}_{\mathcal{B}}[\|\Delta g(\tau|\theta_t)\|^2] - \beta^2 \|\nabla J(\theta_{t-1}) - \nabla J(\theta_t)\|^2 \\ &\quad + \frac{(1 - \beta)^2 \sigma^2}{B} \\ &\leq \beta^2 \|\Delta v_{t-1}\|^2 + \frac{\beta^2}{B^2} \sum_{\tau \in \mathcal{B}_t} \mathbb{E}_{\mathcal{B}}[\|\Delta g(\tau|\theta_t)\|^2] + \frac{(1 - \beta)^2}{B} \sigma^2, \end{aligned} \tag{10}$$

where the first inequality comes from the triangle inequality then we ignore the non-negative terms to arrive at the second inequality.

Additionally, Lemma 6.1 in Xu et al. (2019a) shows that

$$\text{Var}[\omega(\tau|\theta_t, \theta_{t-1})] \leq C_\omega \|\theta_t - \theta_{t-1}\|^2, \tag{11}$$

where  $C_\omega := H(2HG^2 + M)(W + 1)$ .

Using (11) we have

$$\begin{aligned}
 \mathbb{E}_{\mathcal{B}} \left[ \|\Delta g(\tau|\theta_t)\|^2 \right] &= \mathbb{E}_{\mathcal{B}} \left[ \|g(\tau|\theta_t) - \omega(\tau|\theta_t, \theta_{t-1})g(\tau|\theta_{t-1})\|^2 \right] \\
 &= \mathbb{E}_{\mathcal{B}} \left[ \|[1 - \omega(\tau|\theta_t, \theta_{t-1})]g(\tau|\theta_{t-1}) + (g(\tau|\theta_t) - g(\tau|\theta_{t-1}))\|^2 \right] \\
 &\leq \mathbb{E}_{\mathcal{B}} \left[ \|[1 - \omega(\tau|\theta_t, \theta_{t-1})]g(\tau|\theta_{t-1})\|^2 \right] + \mathbb{E}_{\mathcal{B}} \left[ \|g(\tau|\theta_t) - g(\tau|\theta_{t-1})\|^2 \right] \\
 &\stackrel{(\star)}{\leq} C_g^2 \mathbb{E}_{\mathcal{B}} \left[ \|1 - \omega(\tau|\theta_t, \theta_{t-1})\|^2 \right] + L_g^2 \|\theta_t - \theta_{t-1}\|^2 \\
 &\stackrel{(\star\star)}{=} C_g^2 \text{Var}[\omega(\tau|\theta_t, \theta_{t-1})] + L_g^2 \|\theta_t - \theta_{t-1}\|^2 \\
 &\stackrel{(11)}{\leq} (C_g^2 C_\omega + L_g^2) \|\theta_t - \theta_{t-1}\|^2,
 \end{aligned}$$

where  $L_g := \frac{HM(R+|b|)}{(1-\gamma)}$ ,  $C_g := \frac{HG(R+|b|)}{(1-\gamma)}$ , and  $b$  is a baseline reward. Here,  $(\star)$  comes from Lemma 3.1 and  $(\star\star)$  is from Lemma 1 in Cortes et al. (2010).

Plugging the last estimate into (10) yields

$$\mathbb{E}_{\mathcal{B}, \hat{\mathcal{B}}} [\|\Delta v_t\|^2] \leq \beta^2 \|\Delta v_{t-1}\|^2 + \frac{\beta^2 (C_g^2 C_\omega + L_g^2)}{B} \|\theta_t - \theta_{t-1}\|^2 + \frac{(1-\beta)^2}{B} \sigma^2, \quad (12)$$

which is (6), where  $\bar{C} := C_g^2 C_\omega + L_g^2$ . □

## A.2 Proof of Lemma 4.2: Key Estimate of Algorithm 1

Similar to the proof of Lemma 5 in Tran-Dinh et al. (2019b), from the update in Algorithm 1, we have  $\theta_{t+1} = (1-\gamma)\theta_t + \gamma\hat{\theta}_{t+1}$ , which leads to  $\theta_{t+1} - \theta_t = \gamma(\hat{\theta}_{t+1} - \theta_t)$ . Combining this expression and the  $L$ -smoothness of  $J(\theta)$  in Lemma 3.1, we have

$$\begin{aligned}
 J(\theta_{t+1}) &\geq J(\theta_t) + [\nabla J(\theta_t)]^\top (\theta_{t+1} - \theta_t) - \frac{L}{2} \|\theta_{t+1} - \theta_t\|^2 \\
 &= J(\theta_t) + \alpha [\nabla J(\theta_t)]^\top (\hat{\theta}_{t+1} - \theta_t) - \frac{L\alpha^2}{2} \|\hat{\theta}_{t+1} - \theta_t\|^2.
 \end{aligned} \quad (13)$$

From the convexity of  $Q$ , we have

$$Q(\theta_{t+1}) \leq (1-\alpha)Q(\theta_t) + \alpha Q(\hat{\theta}_{t+1}) \leq Q(\theta_t) + \alpha \nabla Q(\hat{\theta}_{t+1})^\top (\hat{\theta}_{t+1} - \theta_t), \quad (14)$$

where  $\nabla Q(\hat{\theta}_{t+1})$  is a subgradient of  $Q$  at  $\hat{\theta}_{t+1}$ .

By the optimality condition of  $\hat{\theta}_{t+1} = \text{prox}_{\eta Q}(\theta_t + \eta v_t)$ , we can show that  $\nabla Q(\hat{\theta}_{t+1}) = v_t - \frac{1}{\eta}(\hat{\theta}_{t+1} - \theta_t)$  for some  $\nabla Q(\hat{\theta}_{t+1}) \in \partial Q(\hat{\theta}_{t+1})$  where  $\partial Q$  is the subdifferential of  $Q$  at  $\hat{\theta}_{t+1}$ . Plugging this into (14), we get

$$Q(\theta_{t+1}) \leq Q(\theta_t) + \alpha v_t^\top (\hat{\theta}_{t+1} - \theta_t) - \frac{\alpha}{\eta} \|\hat{\theta}_{t+1} - \theta_t\|^2. \quad (15)$$

Subtracting (15) from (13), we obtain

$$\begin{aligned}
 F(\theta_{t+1}) &\geq F(\theta_t) + \alpha [\nabla J(\theta_t) - v_t]^\top (\hat{\theta}_{t+1} - \theta_t) + \left( \frac{\alpha}{\eta} - \frac{L\alpha^2}{2} \right) \|\hat{\theta}_{t+1} - \theta_t\|^2 \\
 &= F(\theta_t) - \alpha [v_t - \nabla J(\theta_t)]^\top (\hat{\theta}_{t+1} - \theta_t) + \left( \frac{\alpha}{\eta} - \frac{L\alpha^2}{2} \right) \|\hat{\theta}_{t+1} - \theta_t\|^2.
 \end{aligned} \quad (16)$$

Using the fact that

$$\begin{aligned}
 [v_t - \nabla J(\theta_t)]^\top (\hat{\theta}_{t+1} - \theta_t) &= \frac{1}{2} \|v_t - \nabla J(\theta_t)\|^2 + \frac{1}{2} \|\hat{\theta}_{t+1} - \theta_t\|^2 \\
 &\quad - \frac{1}{2} \|v_t - \nabla J(\theta_t) - (\hat{\theta}_{t+1} - \theta_t)\|^2,
 \end{aligned}$$

and ignoring the non-negative term  $\frac{1}{2}\|v_t - \nabla J(\theta_t) - (\widehat{\theta}_{t+1} - \theta_t)\|^2$ , we can rewrite (16) as

$$F(\theta_{t+1}) \geq F(\theta_t) - \frac{\alpha}{2} \|\nabla J(\theta_t) - v_t\|^2 + \left( \frac{\alpha}{\eta} - \frac{L\alpha^2}{2} - \frac{\alpha}{2} \right) \|\widehat{\theta}_{t+1} - \theta_t\|^2.$$

Taking the total expectation over the entire history  $\mathcal{F}_{t+1}$ , we obtain

$$\mathbb{E}[F(\theta_{t+1})] \geq \mathbb{E}[F(\theta_t)] - \frac{\alpha}{2} \mathbb{E}[\|\nabla J(\theta_t) - v_t\|^2] + \left( \frac{\alpha}{\eta} - \frac{L\alpha^2}{2} - \frac{\alpha}{2} \right) \mathbb{E}[\|\widehat{\theta}_{t+1} - \theta_t\|^2]. \quad (17)$$

From the definition of the gradient mapping (3), we have

$$\eta \|\mathcal{G}_\eta(\theta_t)\| = \|\text{prox}_{\eta Q}(\theta_t + \eta \nabla J(\theta_t)) - \theta_t\|.$$

Applying the triangle inequality, we can derive

$$\begin{aligned} \eta \|\mathcal{G}_\eta(\theta_t)\| &\leq \|\widehat{\theta}_{t+1} - \theta_t\| + \|\text{prox}_{\eta Q}(\theta_t + \eta \nabla J(\theta_t)) - \widehat{\theta}_{t+1}\| \\ &= \|\widehat{\theta}_{t+1} - \theta_t\| + \|\text{prox}_{\eta Q}(\theta_t + \eta \nabla J(\theta_t)) - \text{prox}_{\eta Q}(\theta_t + \eta v_t)\| \\ &\leq \|\widehat{\theta}_{t+1} - \theta_t\| + \eta \|v_t - \nabla J(\theta_t)\|. \end{aligned}$$

Taking the full expectation over the entire history  $\mathcal{F}_{t+1}$  yields

$$\eta^2 \mathbb{E}[\|\mathcal{G}_\eta(\theta_t)\|^2] \leq 2\mathbb{E}[\|\widehat{\theta}_{t+1} - \theta_t\|^2] + 2\eta^2 \mathbb{E}[\|v_t - \nabla J(\theta_t)\|^2].$$

Multiply this inequality by  $-\frac{\alpha}{2}$  and add to (17), we arrive at

$$\begin{aligned} \mathbb{E}[F(\theta_{t+1})] &\geq \mathbb{E}[F(\theta_t)] + \frac{\eta^2 \alpha}{2} \mathbb{E}[\|\mathcal{G}_\eta(\theta_t)\|^2] - \frac{\alpha}{2} (1 + 2\eta^2) \mathbb{E}[\|v_t - \nabla J(\theta_t)\|^2] \\ &\quad + \frac{\alpha}{2} \left( \frac{2}{\eta} - L\alpha - 3 \right) \mathbb{E}[\|\widehat{\theta}_{t+1} - \theta_t\|^2], \end{aligned}$$

which can be rewritten as

$$\mathbb{E}[F(\theta_{t+1})] \geq \mathbb{E}[F(\theta_t)] + \frac{\eta^2 \alpha}{2} \mathbb{E}[\|\mathcal{G}_\eta(\theta_t)\|^2] - \frac{\xi}{2} \mathbb{E}[\|v_t - \nabla J(\theta_t)\|^2] + \frac{\zeta}{2} \mathbb{E}[\|\widehat{\theta}_{t+1} - \theta_t\|^2],$$

where  $\xi := \alpha(1 + 2\eta^2)$  and  $\zeta := \alpha \left( \frac{2}{\eta} - L\alpha - 3 \right)$  which is exactly (7).  $\square$

### A.3 Proof of Theorem 4.1: Key Bound on the Gradient Mapping

Firstly, using the identity  $\theta_{t+1} - \theta_t = \gamma(\widehat{\theta}_{t+1} - \theta_t)$ , taking the total expectation over the entire history  $\mathcal{F}_{t+1}$ , we can rewrite (6) as

$$\begin{aligned} \mathbb{E}[\|v_{t+1} - \nabla J(\theta_{t+1})\|^2] &\leq \beta^2 \mathbb{E}[\|v_t - \nabla J(\theta_t)\|^2] + \frac{\beta^2 \bar{C}}{B} \mathbb{E}[\|\theta_{t+1} - \theta_t\|^2] + \frac{(1-\beta)^2}{B} \sigma^2 \\ &= \beta^2 \mathbb{E}[\|v_t - \nabla J(\theta_t)\|^2] + \frac{\beta^2 \bar{C} \alpha^2}{B} \mathbb{E}[\|\widehat{\theta}_{t+1} - \theta_t\|^2] + \frac{(1-\beta)^2}{B} \sigma^2. \end{aligned} \quad (18)$$

Multiply (18) by  $-\frac{\kappa}{2}$  for some  $\kappa > 0$ , then add to (7), we have

$$\begin{aligned} &\mathbb{E}[F(\theta_{t+1})] - \frac{\kappa}{2} \mathbb{E}[\|v_{t+1} - \nabla J(\theta_{t+1})\|^2] \\ \geq &\mathbb{E}[F(\theta_t)] - \frac{(\kappa\beta^2 + \xi)}{2} \mathbb{E}[\|v_t - \nabla J(\theta_t)\|^2] + \frac{\eta^2 \alpha}{2} \mathbb{E}[\|\mathcal{G}_\eta(\theta_t)\|^2] + \frac{1}{2} \left( \zeta - \frac{\kappa\beta^2 \bar{C} \alpha^2}{B} \right) \mathbb{E}[\|\widehat{\theta}_{t+1} - \theta_t\|^2] \\ &\quad - \frac{\kappa(1-\beta)^2 \sigma^2}{2B} \\ = &\mathbb{E}[F(\theta_t)] - \frac{\kappa}{2} \mathbb{E}[\|v_t - \nabla J(\theta_t)\|^2] + \frac{\eta^2 \alpha}{2} \mathbb{E}[\|\mathcal{G}_\eta(\theta_t)\|^2] - \frac{[\xi - \kappa(1-\beta^2)]}{2} \mathbb{E}[\|v_t - \nabla J(\theta_t)\|^2] \\ &\quad + \frac{1}{2} \left( \zeta - \frac{\kappa\beta^2 \bar{C} \alpha^2}{B} \right) \mathbb{E}[\|\widehat{\theta}_{t+1} - \theta_t\|^2] - \frac{\kappa(1-\beta)^2 \sigma^2}{2B}. \end{aligned}$$

Let us define  $\bar{F}(\theta_t) := \mathbb{E}[F(\theta_t)] - \frac{\kappa}{2}\mathbb{E}[\|v_t - \nabla J(\theta_{t+1})\|^2]$ . Then, the last inequality can be written as

$$\begin{aligned} \bar{F}(\theta_{t+1}) &\geq \bar{F}(\theta_t) + \frac{\eta^2\alpha}{2}\mathbb{E}[\|\mathcal{G}_\eta(\theta_t)\|^2] - \frac{[\xi - \kappa(1-\beta^2)]}{2}\mathbb{E}[\|v_t - \nabla J(\theta_t)\|^2] \\ &\quad - \frac{\kappa(1-\beta^2)\sigma^2}{2B} + \frac{1}{2}\left(\zeta - \frac{\kappa\beta^2\bar{C}\alpha^2}{B}\right)\mathbb{E}[\|\hat{\theta}_{t+1} - \theta_t\|^2]. \end{aligned} \quad (19)$$

Suppose that  $\eta, \alpha, \beta$  are chosen such that

$$\frac{2}{\eta} - L\alpha - 3 \geq \frac{\kappa\beta^2\bar{C}\alpha}{B} > 0 \quad \text{and} \quad \alpha(1 + 2\eta^2) \leq \kappa(1 - \beta^2). \quad (20)$$

Then, we have  $\zeta \geq \frac{\kappa\beta^2\bar{C}\alpha^2}{B}$  and  $\xi \leq \kappa(1 - \beta^2)$ . By ignoring the non-negative terms in (19), we can rewrite it as

$$\bar{F}(\theta_{t+1}) \geq \bar{F}(\theta_t) + \frac{\eta^2\alpha}{2}\mathbb{E}[\|\mathcal{G}_\eta(\theta_t)\|^2] - \frac{\kappa(1 - \beta^2)\sigma^2}{2B}.$$

Summing the above inequality for  $t = 0, \dots, m$ , we obtain

$$\bar{F}(\theta_{m+1}) \geq \bar{F}(\theta_0) + \frac{\eta^2\alpha}{2}\sum_{t=0}^m\mathbb{E}[\|\mathcal{G}_\eta(\theta_t)\|^2] - \frac{\kappa(m+1)(1 - \beta^2)\sigma^2}{2B}. \quad (21)$$

Rearranging terms and multiply both sides by  $\frac{2}{\eta^2\alpha}$ , (21) becomes

$$\sum_{t=0}^m\mathbb{E}[\|\mathcal{G}_\eta(\theta_t)\|^2] \leq \frac{2}{\eta^2\alpha}[\bar{F}(\theta_{m+1}) - \bar{F}(\theta_0)] + \frac{\kappa(m+1)(1 - \beta^2)\sigma^2}{\eta^2\alpha B}. \quad (22)$$

Note that

$$\bar{F}(\theta_0) = F(\theta_0) - \frac{\kappa}{2}\mathbb{E}[\|v_0 - \nabla J(\theta_0)\|^2] \geq F(\theta_0) - \frac{\kappa\sigma^2}{2N},$$

and  $\bar{F}(\theta_{m+1}) = F(\theta_{m+1}) - \frac{\kappa}{2}\mathbb{E}[\|v_{m+1} - \nabla J(\theta_{m+1})\|^2] \leq F(\theta_{m+1})$ . Using these estimate in (22), we obtain

$$\begin{aligned} \sum_{t=0}^m\mathbb{E}[\|\mathcal{G}_\eta(\theta_t)\|^2] &\leq \frac{2}{\eta^2\alpha}[F(\theta_{m+1}) - F(\theta_0)] + \frac{\kappa\sigma^2}{\eta^2\alpha N} + \frac{\kappa(m+1)(1 - \beta^2)\sigma^2}{\eta^2\alpha B} \\ &= \frac{2}{\eta^2\alpha}[F(\theta_{m+1}) - F(\theta_0)] + \frac{(m+1)\kappa\sigma^2}{\eta^2\alpha}\left[\frac{1}{N(m+1)} + \frac{(1 - \beta^2)}{B}\right]. \end{aligned}$$

Multiplying both sides by  $\frac{1}{m+1}$ , we have

$$\frac{1}{m+1}\sum_{t=0}^m\mathbb{E}[\|\mathcal{G}_\eta(\theta_t)\|^2] \leq \frac{2}{\eta^2\alpha(m+1)}[F(\theta_{m+1}) - F(\theta_0)] + \frac{\kappa\sigma^2}{\eta^2\alpha}\left[\frac{1}{N(m+1)} + \frac{(1 - \beta^2)}{B}\right]. \quad (23)$$

Now we choose  $\beta := 1 - \frac{\sqrt{B}}{\sqrt{N(m+1)}}$  so that the right-hand side of (23) is minimized. Note that if  $1 \leq B \leq N(m+1)$ , then  $\beta \in [0, 1)$ .

Let us choose  $\eta := \frac{2}{4+L\alpha} \leq \frac{1}{2}$  which means  $\zeta := \frac{2}{\eta} - L\alpha - 3 = 1$ . We can satisfy the first condition of (20) by choosing  $0 < \alpha \leq \frac{B}{\kappa\bar{C}}$ .

Besides, the second condition in (20) holds if  $0 < \alpha \leq \frac{\kappa(1-\beta^2)}{1+2\eta^2}$ . Since we have  $\eta \leq \frac{1}{2}$  which leads to  $1 + 2\eta^2 \leq \frac{3}{2}$  and using  $1 - \beta^2 \geq 1 - \beta = \frac{B^{1/2}}{N^{1/2}(m+1)^{1/2}}$  we derive the condition for  $\alpha$  as

$$0 < \alpha \leq \frac{2\kappa\sqrt{B}}{3\sqrt{N(m+1)}}.$$

Therefore, the overall condition for  $\alpha$  is given as

$$0 < \alpha \leq \min\left\{1, \frac{B}{\kappa\bar{C}}, \frac{2\kappa\sqrt{B}}{3\sqrt{N(m+1)}}\right\}.$$

If we choose  $\kappa := \frac{\sqrt{3[NB(m+1)]^{1/4}}}{\sqrt{2C}}$ , then we can update  $\alpha$  as

$$\alpha := \frac{\hat{c}\sqrt{2}B^{3/4}}{\sqrt{3C}[N(m+1)]^{1/4}}. \quad (24)$$

Using  $1 \leq B \leq N(m+1)$ , we can bound  $\alpha \leq \hat{c}\sqrt{\frac{2B}{3C}}$  then we can choose  $\hat{c} \in \left(0, \sqrt{\frac{3C}{2B}}\right]$  so that  $\gamma \in (0, 1]$ .

With all the choices of  $\beta$ ,  $\eta$ ,  $\alpha$ , and  $\kappa$  above, if we let the output  $\tilde{\theta}_T$  be selected uniformly at random from  $\{\theta_t\}_{t=0}^m$ , then we have

$$\begin{aligned} \mathbb{E} \left[ \|\mathcal{G}_\eta(\tilde{\theta}_T)\|^2 \right] &= \frac{1}{m+1} \sum_{t=0}^m \mathbb{E} \left[ \|\mathcal{G}_\eta(\theta_t)\|^2 \right] \\ &\leq \frac{\sqrt{3C}N^{1/4}}{\eta^2 \hat{c} \sqrt{2} [B(m+1)]^{3/4}} [F(\theta_{m+1}) - F(\theta_0)] + \frac{3\sigma^2}{\eta^2 [BN(m+1)]^{1/2}}. \end{aligned} \quad (25)$$

Note that  $\eta = \frac{2}{4+L\alpha}$  and since  $\alpha \leq 1$  we have  $\frac{1}{\eta^2} \leq \frac{(4+L)^2}{4}$ . Plugging these into (25), we obtain

$$\begin{aligned} \mathbb{E} \left[ \|\mathcal{G}_\eta(\tilde{\theta}_T)\|^2 \right] &= \frac{1}{m+1} \sum_{t=0}^m \mathbb{E} \left[ \|\mathcal{G}_\eta(\theta_t)\|^2 \right] \\ &\leq \frac{(4+L)^2 \sqrt{3C} N^{1/4}}{4\hat{c}\sqrt{2}[B(m+1)]^{3/4}} [F(\theta_{m+1}) - F(\theta_0)] + \frac{3(4+L)^2 \sigma^2}{4[BN(m+1)]^{1/2}} \\ &\leq \frac{(4+L)^2 \sqrt{3C} N^{1/4}}{4\hat{c}\sqrt{2}[B(m+1)]^{3/4}} [F^* - F(\theta_0)] + \frac{3(4+L)^2 \sigma^2}{4[BN(m+1)]^{1/2}}, \end{aligned} \quad (26)$$

where we use the fact that  $F(\theta_{m+1}) \leq F^*$ .  $\square$

#### A.4 Proof of Corollary 4.1: Trajectory Complexity Bound of Algorithm 1 and Algorithm 2

If we fix a batch size  $B \in \mathbb{N}_+$  and choose  $N := \tilde{c}\sigma^{8/3} [B(m+1)]^{1/3}$  for some  $\tilde{c} > 0$ , (26) is equivalent to

$$\begin{aligned} \mathbb{E} \left[ \|\mathcal{G}_\eta(\tilde{\theta}_T)\|^2 \right] &\leq \frac{(4+L)^2 \sqrt{3C} \tilde{c}^{1/4} \sigma^{2/3}}{4\hat{c}\sqrt{2}[B(m+1)]^{2/3}} [F^* - F(\bar{\theta}^{(0)})] + \frac{3(4+L)^2 \sigma^{2/3}}{4\tilde{c}^{1/2}[B(m+1)]^{2/3}} \\ &= \left[ \frac{(4+L)^2 \sqrt{3C} \tilde{c}^{1/4}}{4\hat{c}\sqrt{2}} [F^* - F(\bar{\theta}^{(0)})] + \frac{3(4+L)^2}{4\tilde{c}^{1/2}} \right] \frac{\sigma^{2/3}}{[B(m+1)]^{2/3}} \\ &= \frac{\Psi_0 \sigma^{2/3}}{[B(m+1)]^{2/3}}, \end{aligned}$$

where we define

$$\Psi_0 := \left[ \frac{(4+L)^2 \sqrt{3C} \tilde{c}^{1/4}}{4\hat{c}\sqrt{2}} [F^* - F(\bar{\theta}^{(0)})] + \frac{3(4+L)^2}{4\tilde{c}^{1/2}} \right]. \quad (27)$$

Therefore, for any  $\varepsilon > 0$ , to guarantee  $\mathbb{E} \left[ \|\mathcal{G}_\eta(\tilde{\theta}_T)\|^2 \right] \leq \varepsilon^2$ , we need  $\frac{\Psi_0 \sigma^{2/3}}{[B(m+1)]^{2/3}} = \varepsilon^2$  which leads to the total number of iterations

$$T = m + 1 = \frac{\Psi_0^{3/2} \sigma}{B\varepsilon^3} = \mathcal{O} \left( \frac{1}{\varepsilon^3} \right).$$

The total number of proximal operations  $\text{prox}_{\eta Q}$  is also  $\mathcal{O} \left( \frac{1}{\varepsilon^3} \right)$ . In addition, the total number of trajectories is at most

$$\begin{aligned} N + 2B(m+1) &= \tilde{c}\sigma^{8/3} [B(m+1)]^{1/3} + \frac{2\Psi_0 \sigma}{\varepsilon^3} \\ &= \tilde{c}\sigma^{8/3} \frac{\Psi_0^{1/3} \sigma^{1/3}}{\varepsilon} + \frac{2\Psi_0 \sigma}{\varepsilon^3} \\ &= \mathcal{O} \left( \frac{1}{\varepsilon} + \frac{1}{\varepsilon^3} \right) = \mathcal{O} \left( \frac{1}{\varepsilon^3} \right). \end{aligned}$$

This proves our the complexity of Algorithm 1.

Next, let us denote the superscript  $(s)$  when the current stage is  $s$  for  $s = 0, \dots, S-1$ . Note that from the first inequality of (26), for any stage  $s = 0, \dots, S-1$ , the following holds

$$\frac{1}{m+1} \sum_{t=0}^m \mathbb{E} \left[ \|\mathcal{G}_\eta(\theta_t^{(s)})\|^2 \right] \leq \frac{(4+L)^2 \sqrt{3\bar{C}} N^{1/4}}{4\hat{c}\sqrt{2}[B(m+1)]^{3/4}} \left[ F(\theta_{m+1}^{(s)}) - F(\theta_0^{(s)}) \right] + \frac{3(4+L)^2 \sigma^2}{4[B\bar{N}(m+1)]^{1/2}}.$$

Summing for  $s = 0, \dots, S-1$  and multiply both sides by  $\frac{1}{S}$  yields

$$\begin{aligned} \frac{1}{S(m+1)} \sum_{s=0}^{S-1} \sum_{t=0}^m \mathbb{E} \left[ \|\mathcal{G}_\eta(\theta_t^{(s)})\|^2 \right] &\leq \frac{(4+L)^2 \sqrt{3\bar{C}} N^{1/4}}{4\hat{c}\sqrt{2}[B(m+1)]^{3/4} S} \left[ F(\theta_{m+1}^{(S-1)}) - F(\theta_0^{(0)}) \right] + \frac{3(4+L)^2 \sigma^2}{4[B\bar{N}(m+1)]^{1/2} S} \\ &\leq \frac{(4+L)^2 \sqrt{3\bar{C}} N^{1/4}}{4\hat{c}\sqrt{2}[B(m+1)]^{3/4} S} \left[ F^* - F(\theta_0^{(0)}) \right] + \frac{3(4+L)^2 \sigma^2}{4[B\bar{N}(m+1)]^{1/2} S}, \end{aligned} \quad (28)$$

where we use  $F(\theta_{m+1}^{(S-1)}) \leq F^*$  again.

If we also fix a batch size  $B \in \mathbb{N}_+$  and choose  $N := \tilde{c}\sigma^{8/3} [B(m+1)]^{1/3}$  for some  $\tilde{c} > 0$ , and select  $\tilde{\theta}_T$  uniformly random from  $\{\theta_t^{(s)}\}_{t=0, \dots, m}^{s=1, \dots, S}$ , then, similar to (A.4), (28) can be written as

$$\begin{aligned} \mathbb{E} \left[ \|\mathcal{G}_\eta(\tilde{\theta}_T)\|^2 \right] &= \frac{1}{S(m+1)} \sum_{s=0}^{S-1} \sum_{t=0}^m \mathbb{E} \left[ \|\mathcal{G}_\eta(\theta_t^{(s)})\|^2 \right] \\ &\leq \frac{(4+L)^2 \sqrt{3\bar{C}} \tilde{c}^{1/4} \sigma^{2/3}}{4\hat{c}\sqrt{2}[B(m+1)]^{2/3} S} \left[ F^* - F(\theta_0^{(0)}) \right] + \frac{3(4+L)^2 \sigma^{2/3}}{4\tilde{c}^{1/2}[B(m+1)]^{2/3} S} \\ &= \left[ \frac{(4+L)^2 \sqrt{3\bar{C}} \tilde{c}^{1/4}}{4\hat{c}\sqrt{2}} \left[ F^* - F(\theta_0^{(0)}) \right] + \frac{3(4+L)^2}{4\tilde{c}^{1/2}} \right] \frac{\sigma^{2/3}}{[B(m+1)]^{2/3} S} \\ &\leq \frac{\Psi_0 \sigma^{2/3}}{[SB(m+1)]^{2/3}}, \end{aligned}$$

where we use  $\Psi_0$  defined in (27) and  $\frac{1}{S} \leq \frac{1}{S^{2/3}}$  for any  $S \geq 1$ .

Therefore, to guarantee  $\mathbb{E} \left[ \|\mathcal{G}_\eta(\tilde{\theta}_T)\|^2 \right] \leq \varepsilon^2$  for any  $\varepsilon > 0$ , we need  $\frac{\Psi_0 \sigma^{2/3}}{[SB(m+1)]^{2/3}} = \varepsilon^2$  which leads to the total number of iterations

$$T = S(m+1) = \frac{\Psi_0^{3/2} \sigma}{B\varepsilon^3} = \mathcal{O} \left( \frac{1}{\varepsilon^3} \right).$$

The total number of proximal operations  $\text{prox}_{\eta Q}$  is also  $\mathcal{O} \left( \frac{1}{\varepsilon^3} \right)$ . In addition, the total number of trajectories is at most

$$\begin{aligned} S[N + 2B(m+1)] &= S \left[ \tilde{c}\sigma^{8/3} [B(m+1)]^{1/3} + \frac{2\Psi_0\sigma}{\varepsilon^3} \right] \\ &= S \left[ \tilde{c}\sigma^{8/3} \frac{\Psi_0^{1/3} \sigma^{1/3}}{\varepsilon} + \frac{2\Psi_0\sigma}{\varepsilon^3} \right] \\ &= \mathcal{O} \left( \frac{1}{\varepsilon} + \frac{1}{\varepsilon^3} \right) = \mathcal{O} \left( \frac{1}{\varepsilon^3} \right), \text{ for any } S \geq 1. \end{aligned}$$

Hence, we obtain the conclusion of Corollary 4.1.  $\square$

## B Configurations of Algorithms in Section 5

Let us describe in detail the configuration of our experiments in Section 5. We set  $\beta := 0.99$  for HSPGA and  $\alpha := 0.99$  for ProxHSPGA in all experiments. To choose the learning rate, we conduct a grid search over different choices. For `Acrobot-v1`, `Cart pole-v0`, and `Mountain Car-v0` environments, we use the grid containing  $\{0.0005, 0.001, 0.0025, 0.005, 0.0075, 0.01\}$ . Meanwhile, we use  $\{0.0005, 0.00075, 0.001, 0.0025, 0.005\}$  for the remaining environments. The snapshot batch-sizes are also chosen from  $\{10, 25, 50, 100\}$  while the mini-batch sizes are selected from  $\{3, 5, 10, 15, 20, 25\}$ . More details about the selected parameters for each experiment are shown in Table 2.

Table 2: The configuration of different algorithms on discrete and continuous control environments

| Environment                   | Algorithm | Policy Network                    | Discount Factor $\gamma$ | Trajectory Length H | Minibatch Size | Snapshot Batchsize | Learning Rate        | Epoch Length $m$ |
|-------------------------------|-----------|-----------------------------------|--------------------------|---------------------|----------------|--------------------|----------------------|------------------|
| CartPole-v0                   | GPOMDP    | $4 \times 8 \times 2$             | 0.99                     | 200                 | 10             |                    | $10^{-3}$            |                  |
|                               | SVRPG     |                                   |                          |                     | 10             | 25                 | $5 \times 10^{-3}$   | 3                |
|                               | HSPGA     |                                   |                          |                     | 5              | 25                 | $5 \times 10^{-3}$   | 3                |
| Acrobot-v1                    | GPOMDP    | $6 \times 16 \times 3$            | 0.999                    | 500                 | 10             |                    | $2.5 \times 10^{-3}$ |                  |
|                               | SVRPG     |                                   |                          |                     | 5              | 10                 | $5 \times 10^{-3}$   | 3                |
|                               | HSPGA     |                                   |                          |                     | 3              | 10                 | $5 \times 10^{-3}$   | 3                |
| MountainCar-v0                | GPOMDP    | $2 \times 8 \times 1$             | 0.999                    | 1000                | 25             |                    | $5 \times 10^{-3}$   |                  |
|                               | SVRPG     |                                   |                          |                     | 10             | 50                 | $7.5 \times 10^{-3}$ | 3                |
|                               | HSPGA     |                                   |                          |                     | 5              | 50                 | $7.5 \times 10^{-3}$ | 3                |
| RoboschoolInvertedPendulum-v1 | GPOMDP    | $5 \times 16 \times 1$            | 0.999                    | 1000                | 20             |                    | $7.5 \times 10^{-4}$ |                  |
|                               | SVRPG     |                                   |                          |                     | 10             | 50                 | $10^{-3}$            | 3                |
|                               | HSPGA     |                                   |                          |                     | 5              | 50                 | $10^{-3}$            | 3                |
|                               | ProxHSPGA |                                   |                          |                     | 5              | 50                 | $10^{-3}$            | 3                |
| Swimmer-v2                    | GPOMDP    | $8 \times 32 \times 32 \times 2$  | 0.99                     | 500                 | 50             |                    | $5 \times 10^{-4}$   |                  |
|                               | SVRPG     |                                   |                          |                     | 5              | 50                 | $5 \times 10^{-4}$   | 3                |
|                               | HSPGA     |                                   |                          |                     | 5              | 50                 | $5 \times 10^{-4}$   | 3                |
|                               | ProxHSPGA |                                   |                          |                     | 5              | 50                 | $5 \times 10^{-4}$   | 3                |
| Hopper-v2                     | GPOMDP    | $11 \times 32 \times 32 \times 3$ | 0.99                     | 500                 | 50             |                    | $5 \times 10^{-4}$   |                  |
|                               | SVRPG     |                                   |                          |                     | 5              | 50                 | $5 \times 10^{-4}$   | 3                |
|                               | HSPGA     |                                   |                          |                     | 5              | 50                 | $5 \times 10^{-4}$   | 3                |
|                               | ProxHSPGA |                                   |                          |                     | 5              | 50                 | $5 \times 10^{-4}$   | 3                |
| Walker2d-v2                   | GPOMDP    | $17 \times 32 \times 32 \times 6$ | 0.99                     | 500                 | 50             |                    | $5 \times 10^{-4}$   |                  |
|                               | SVRPG     |                                   |                          |                     | 5              | 50                 | $5 \times 10^{-4}$   | 3                |
|                               | HSPGA     |                                   |                          |                     | 5              | 50                 | $5 \times 10^{-4}$   | 3                |
|                               | ProxHSPGA |                                   |                          |                     | 5              | 50                 | $5 \times 10^{-4}$   | 3                |

## C Additional Numerical Results

Due to space limit in the main text, we show here another evidence on the effect of regularizers to policy optimization problems by carrying out an additional example on other continuous control tasks in Mujoco. The results are presented in Figure 5.

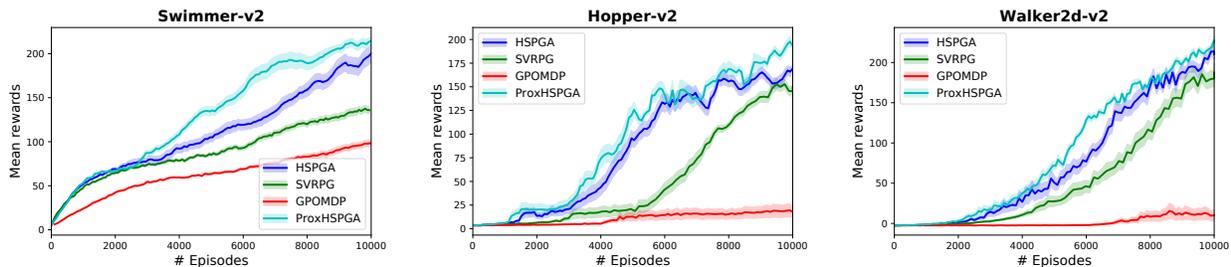

Figure 5: The performance of 4 algorithms on the composite vs. the non-composite settings using several Mujoco environments.

Again, Figure 5 still reveals the benefit of adding a regularizer, which potentially gains more reward than without using regularizer. We believe that the choice of regularizer is also critical and may lead to different performance. We refer to (Liu et al., 2019) for more evidence of using regularizers in reinforcement learning.
